# Supplementary material for: Toward In-Context Teaching: Adapting Examples to Students' Misconceptions
Source: arXiv:2405.04495 source file (2024-05-07)
Supplement: Supplementary file 1 [file secondhalf.pdf]

Timer: 10:00

# Mystery Machine Study

## Chat

**Accuracy of Predictions:**
Streak:

Press **"I Am Ready"** when you are ready to start learning. After that, the **timer** will begin, and you will have **10 minutes** to interact with the teacher and submit guesses. You are encouraged to play around with the interface before beginning.

I Am Ready

Type your message here...

Send

*I'm pretty sure, but not totally confident, that:*

1. *wug is undefined when inputs are* ***divisible by 3***
2. *When wug is defined, b =* ***8***

*--Dr. Smith*

### Make a guess about wug

(1) wug(x) is undefined when input **x** is:

--

(2) when defined, wug(x) computes a***x**+b

where: a=- b=-

Remember: **Multiple guesses** are allowed, and you can get **partial credit** for getting only one part of wug correct. The sooner you have the correct guess for wug, the higher your bonus.

**Calculator** for a***x**+b where:

a=- b=- OR Reset to Guess

x= 0 Result:

You can use this calculator to help you figure out wug; it will not affect your bonus.

Back

Timer: 09:26

# Mystery Machine Study

## Chat

**Accuracy of Predictions:** 1/3
Streak:

Teacher: What is **wug(2)**?

You: 8

Teacher: That's incorrect. **wug(2)=14**. What is **wug(4)**?

You: 20

Teacher: That's correct. What is **wug(6)**?

You: undefined

Teacher: That's incorrect. **wug(6)=26**. What is **wug(8)**?

Type your message here...

Send

*I'm pretty sure, but not totally confident, that:*

1. *wug is undefined when inputs are **divisible by 3***
2. *When wug is defined, b = **8***

*--Dr. Smith*

### Make a guess about wug

(1) wug(x) is undefined when input **x** is:

--

(2) when defined, wug(x) computes a*x+b

where: a=- b=-

Remember: **Multiple guesses** are allowed, and you can get **partial credit** for getting only one part of wug correct. The sooner you have the correct guess for wug, the higher your bonus.

**Calculator** for a*x+b where:

a=3 b=8 OR Reset to Guess

x= 4 Result: 3*x+8=20

You can use this calculator to help you figure out wug; it will not affect your bonus.

Back

# Mystery Machine Study

## Exit Questions

**A) Was Dr. Smith's note right?**

> *I'm pretty sure, but not totally confident, that:*
>
> 1. *wug is undefined when inputs are **divisible by 3***
> 2. *When wug is defined, b = **8***
>
> *--Dr. Smith*

**Hint (1) was:**

○ Correct ○ Incorrect ○ I don't know

**Hint (2) was:**

○ Correct ○ Incorrect ○ I don't know

**B) Did Dr. Smith's note influence what you thought wug did?**

○ Yes ○ No

**C) Was there anything you found confusing or did not understand throughout the study, or any other issues that you encountered?**

Submit

# Mystery Machine Study

You have finished the study. Thank you for participating! Here is your completion code:

The correct answer was:

1. *wug is undefined when inputs are **odd***
2. *When wug is defined, it computes* $a*x+b$ *where* $a$ = ***3*** *and* $b$ = ***8***

If you have questions about this research, please contact us at `alexisro@mit.edu`. We will be in touch about your bonus.
