# Supplementary material for: Toward In-Context Teaching: Adapting Examples to Students' Misconceptions
Source: arXiv:2405.04495 source file (2024-05-07)
Supplement: Supplementary file 2 [file instructions.pdf]

# Mystery Machine Study

## Introduction

By entering your Prolific ID below, you are participating in a study being performed by computer scientists in the MIT Department of Electrical Engineering and Computer Science and are agreeing to the following:

- You must be at least 18 years old to participate. Your participation in this research is voluntary.
- You may decline to answer any or all of the following questions. You may decline further participation, at any time, without adverse consequences.
- Your anonymity is assured; the researchers who have requested your participation will not receive any personal information about you.

Once you click submit, you will not be able to come back to this page.

Enter your Prolific ID:

Submit

# Mystery Machine Study

## Task

### Goal

In this study, we are researching the way that people learn from examples. You will be tasked with learning what a **mystery machine** called **wug** does. This machine takes in numbers and outputs numbers; **wug(x)=y** means that when **wug** takes in number **x**, it outputs **y**. However, it only works for some numbers and is **undefined** for others. Your task is to learn on what inputs **wug** is **undefined**, and when it is defined, **what it does**.

For example, suppose that you were instead learning about a machine **vug** that operated on letters instead of numbers. Suppose you saw the following sequence of examples: **vug(A)=B**, **vug(B)=undefined**, **vug(E)=F**, **vug(I)=J**. This data might suggest that **vug** is **undefined** on consonants and, when defined (on vowels), returns the next letter in the alphabet.

[Next](#)

# Mystery Machine Study

## Task

### Details

You will be interacting with a **teacher** through a chat interface, shown on the right. The teacher will show you examples of what **wug** does on different numbers, first asking you what you think **wug** outputs on a given input, and then providing the true output. Your goal is to figure out what **wug** does as quickly as possible.

Throughout the teaching interaction, you can provide your **guess** of what you think **wug** does through the **sidebar** on the right. Your guess will have two parts:

1. when **wug** is undefined
2. when defined, what it does.

We also provide a **calculator** to help with any calculations you may need for your guess.

You will have **10 minutes** to learn from the teacher. After that, you will no longer be able to learn about **wug** or make guesses. If you get **10 predictions correct in a row** while talking to the teacher *or* go through all the teacher's examples before the 10 minutes are up, you will have the option to **end the interaction early**.

Accuracy of Predictions: 2/3

Streak: 1 2 ○ ○ ○ ○ ○ ○ ○ ○ ○ ○

Teacher

What is wug(0)?

You

Teacher

That's **incorrect**. wug(0)=0 What is wug(1)?

You

Teacher

That's **correct**. What is wug(2)?

You

Teacher

That's **correct**. What is wug(3)?

You

Send

### Make a guess about wug

(1) **wug(x)** is undefined when input x is:

--

(2) when defined, **wug(x)** computes  $a \cdot x + b$

where: a=-- b=--

### Calculator for $a \cdot x + b$ where:

a=-- b=-- OR Reset to Guess

x= 0 Result:

Back

Next

# Mystery Machine Study

## Task

### Bonus

You will receive a base pay of \$4.00 for this study. In addition, based on your performance at the task, you will be compensated with a bonus dependent on:

- Accuracy of guesses for wug:** You will receive a higher bonus the sooner and longer you provide a correct guess for wug. You will receive \$0.05 for every 10 seconds of the teaching interaction that your guess is correct. For example, if you provided the correct guess for wug 1 minute into the teaching interaction and left it unchanged, you would have a correct guess for 9 minutes, or equivalently 540 seconds. Therefore, you would get a bonus of  $\$0.05 * (540/10) = \$2.70$ . You will receive partial compensation if only one of the two parts is correct, or if you have the correct guess submitted for less than 10 seconds.
- Accuracy of outputs for teacher examples:** You will receive up to an additional \$1.00 based on how many of your responses to the teacher are correct. For example, in the example teaching interaction in the right image, the participant gave 2/3 answers to the teacher, and so their bonus would be  $\$1.00 * (2/3) = \$0.67$ .

Therefore, you should aim to provide a guess of what wug does as soon as you think you know, and aim to give the teacher accurate answers. You will not know if the guesses you submit for wug are correct.

Accuracy of Predictions: 2/3  
Streak: 1 2 ○ ○ ○ ○ ○ ○ ○ ○ ○ ○

Teacher

What is wug(○)?

You

Teacher

That's incorrect. wug(○)=○ What is wug(○)?

You

Teacher

That's correct. What is wug(○)?

You

Teacher

That's correct. What is wug(○)?

Send

Make a guess about wug

(1) wug(x) is undefined when input x is:

(2) when defined, wug(x) computes  $a * x + b$   
where:

Calculator for  $a * x + b$  where:

OR

x=  Result:

# Mystery Machine Study

## Task

### Hints about wug

Fortunately, you are not starting from a blank slate. Dr. Smith spent a bunch of time studying this machine. She figured out that when wug is defined, it computes a function of the form  $a*x+b$ , where  $a$  and  $b$  are constant numbers, so you only need to figure out what  $a$  and  $b$  are.

She also left a note with some thoughts:

*I'm pretty sure, but not totally confident, that:*

1. wug is undefined when inputs are **divisible by 3**
2. When wug is defined,  $b = 8$

*--Dr. Smith*

Dr. Smith is quite familiar with wug, so her note should give you a good place to start! But keep in mind that it is possible that she is wrong.

We will provide the note for you throughout learning so that you can refer to it. You can also always come back to the task instructions by using the navigation buttons "Back" and "Next" below.

Back

Next

# Mystery Machine Study

## Task

### Instruction check

You now have all the information to start learning **wug**! Before you start, please answer the following questions. If you are unsure of the answers, we encourage you to read through the task instructions again.

The bonus depends on:

- ☐ (1) Accuracy of predictions I give to the teacher
- ☐ (2) How quickly I guess what wug does
- ☒ Both (1) and (2)

**Correct!** The correct answer is *Both (1) and (2)*.

True or False: Multiple guesses for **wug** are allowed.

- ☒ True
- ☐ False

**Correct!** The correct answer is *True*. Multiple guesses are allowed.

Submit

Press "Next" to enter the chat interface. There, you will have the opportunity to familiarize yourself with the layout **before learning begins and the timer starts**. After you press "I Am Ready" on the next page, you will interact with the teacher for 10 minutes.

Back

Next
